# Supplementary material for: Ultrahigh flexoelectric effect of 3D interconnected porous polymers: modelling and verification
Source: arXiv:2009.03847 source file (2021-03-06)
Supplement: Supplementary file 1 [file Supplementary-Zhang_et_al-0306.pdf]

# Ultrahigh flexoelectric effect of 3D interconnected porous polymers: modelling and verication

Mingyuan Zhang[a,1], Dongze Yan[a,1], Jianxiang Wang[b, c], Li-Hua Shao[a, *]

[a] Institute of Solid Mechanics, Beihang University, Beijing 100191, P.R.China.

[b] Department of Mechanics and Engineering Science, College of Engineering, Peking University, Beijing 100871, P. R. China

[c] CAPT-HEDPS, and IFSA Collaborative Innovation Center of MoE, College of Engineering, Peking University, Beijing 100871, P.R. China.

[1]Contribute equally to this work.

*Corresponding Author: Li-Hua Shao, E-Mail: shaolihua@buaa.edu.cn

## Supplementary Materials

### Sample fabrication

As schematically illustrated in Supplementary Fig. 1, PDMS prepolymer (Sylgard 184A, Dow Corning) and the thermal curing agent (Sylgard 184B, Dow Corning) were mixed at a weight ratio of 10:1, which is denoted as “pre-cured PDMS” here. The commercial sugar cubes ($2\times2\times1$ cm$^3$, Taikoo) with particle sizes of ca. 400-500 μm and salt particles (Macklin) with the sizes ranging from 150 μm to 200 μm were used as sacrificial templates. The sugar cube was used as template directly, whereas the salt particles was mixed with the pre-cured PDMS at a weight ratio of 4:1 as the template. The mixture was filled in a $2\times2\times1$ cm$^3$ cubic mold tightly to form the PDMS-salt templates [1]. The templates (sugar cubes or PDMS-salt templates) were placed in a Petri

dish, and the pre-cured PDMS was poured into the Petri dish until it submerged all of the templates. Then the Petri dish was placed into a vacuum chamber, degassing for 2 h at 80 ℃, which allowed the pre-cured PDMS to infiltrate into the pores of the templates with the assist of capillary force during the polymerization [2]. Afterwards, the as-prepared cured PDMS-template cubes were cut off to remove excess PDMS from the surfaces. Then, the PDMS-template cubes were put in water to dissolve the sugar or salt at 80 ℃ for 2 h using ultrasonic cleaner and following ultrapure water cleaning for 5 times. Finally, the 3D interconnected porous PDMS samples with large pores (sugar template) and small pores (salt template) were obtained after drying in a convection oven (Jinghong DHG-9030A, China) for 2 h at 80 ℃. The truncated pyramid was fabricated by filling the pre-cured PDMS into a mold printed by 3D printer (MakerBot PABH65, USA), and then curing for 3 h at 60 ℃ in the aforementioned convection oven. Afterwards, truncated PDMS pyramid sample was peeled off from the mold. In order to collect the flexoelectric charge effectively, silver conductive epoxy adhesives (MG chemicals 8330) with high electric conductivity and low stiffness were brushed on the top and bottom surfaces of the samples as electrodes. The same salt particles (Macklin) were used as sacrificial templates for the fabrication of porous PVDF. PVDF powder and salt particles were mixed at a weight ratio of 1:1 and mechanically ground to form a uniform

powder. Then the mixture was put in silica mould and heated at 220 ℃ for 20 mins. After cooling to room temperature, the samples were immersed in water (40 ℃) for 72 h to remove the salt particles and obtain the porous α-PVDF (α phase)[3], [4].

Both of PDMS and α-PVDF are free of piezoelectricity theoretically, which have also been measured before the experiment.

**Experimental setup**

The dynamic mechanical analyzer (TA ElectroForce-DMA3200, USA) was used for dynamic uniaxial compression. A low-noise current preamplifier (Stanford Research SR-570, USA) was used to measure and convert the current signal to voltage signal, in which a low noise gain mode and a low-pass filter method were chosen. An electrostatic eliminator (KEYENCE SJ-F036, Japan) was used to remove the electrostatic charge. Finally, the oscilloscope (Tektronix MDO-3034, USA) was used to record the real-time voltage signal.

**Materials characterization**

The microscopic structures were characterized by scanning electron microscope (SEM, HITACHI SU8020, Japan), and the ligament and pore sizes were calculated by averaging the values obtained from ImageJ software. The energy dispersive spectroscopy (EDS, IXRF ATLAS, USA) was used to check the salt residual. The corresponding spectrum of the small pore PDMS is shown in Supplementary Fig. 2, where one can

conclude that most of the salt particles have been removed.

**Calculation of pre-deflection**

Considering that the ligaments in the porous specimen are not straight, we assign a relative pre-deflection coefficient $\delta_0' = \delta_0/\delta$ at the midpoint of the vertical beam. According to the SEM image shown in Supplementary Fig. 4(a) (below) of the porous specimen, there are total 14 unit cells ($n$=14) in the range of the height $H$=6.4 mm. In the theoretical model, the height of the unit cell is $h$=2($l$+$\delta$)=0.46 mm. The pre-defection of a single beam is $\delta_0$, where $\delta_0$=$\delta_0'\delta$, and the axial displacement is $\Delta$, we have

$$\Delta = \frac{H-h}{2n} = 1.42857\mu\text{m}\,.$$

For a curved beam with small deflection, since the arc length is approximately the chord length, according to the Pythagorean theorem, we have

$$\left(\frac{l}{2}\right)^2 - \left(\frac{l-\Delta}{2}\right)^2 = \left(\delta_0'\delta\right)^2 .$$

Therefore, $\delta_0'$ is 0.226. Since the length of the chord is less than the arc length and for simplicity, we take $\delta_0' \approx 0.2$, and find that this value fits the results better.

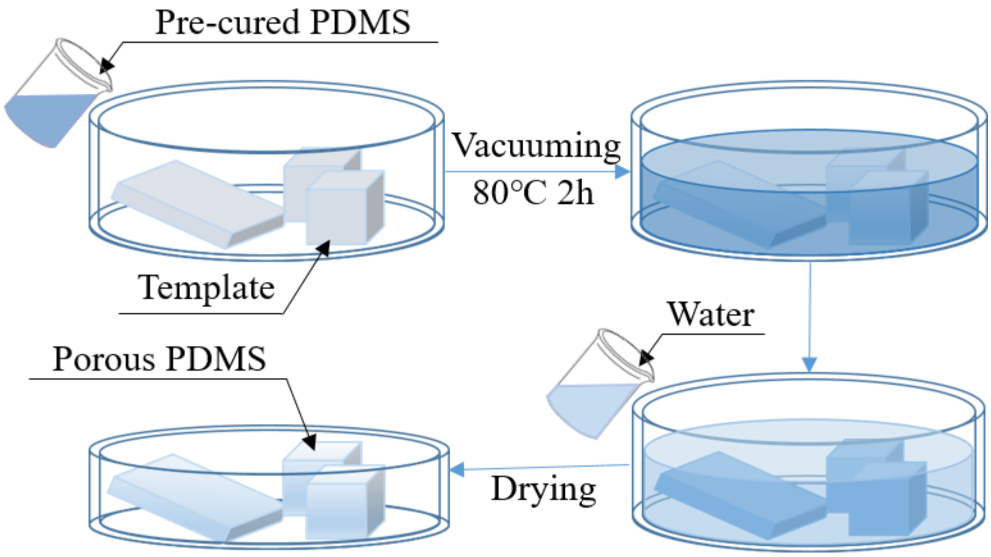


Supplementary Fig. 1. Schematic diagram of the fabrication method of porous PDMS based on direct templating technique.

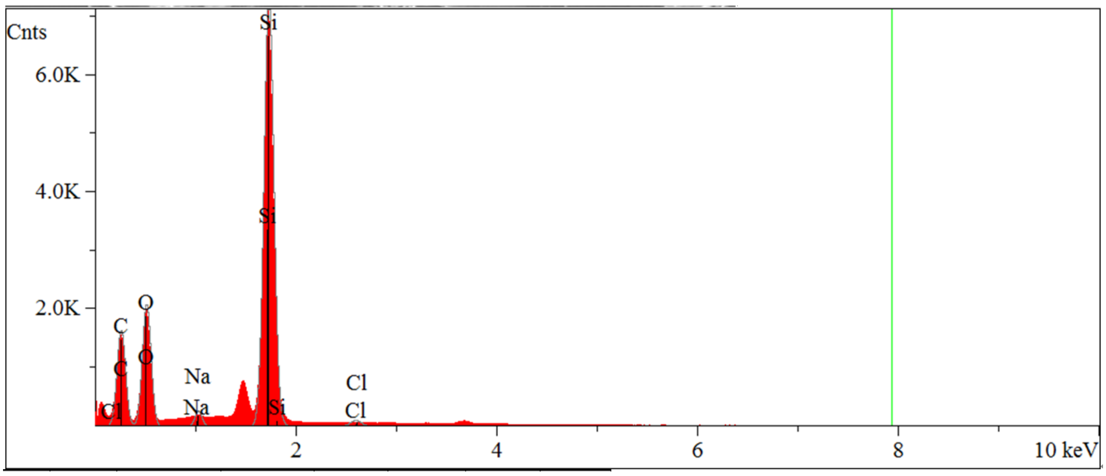


Supplementary Fig. 2. Energy dispersive spectroscopy (EDS) image of small pore PDMS.

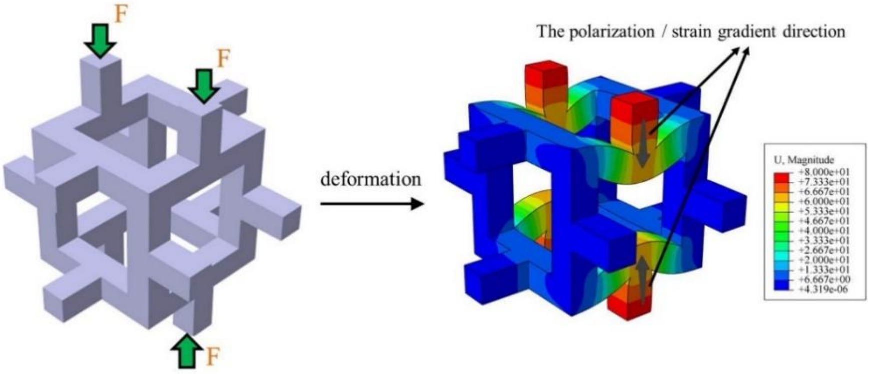


Supplementary Fig. 3. The schematic plot of polarization and strain gradient direction of a unit cell.

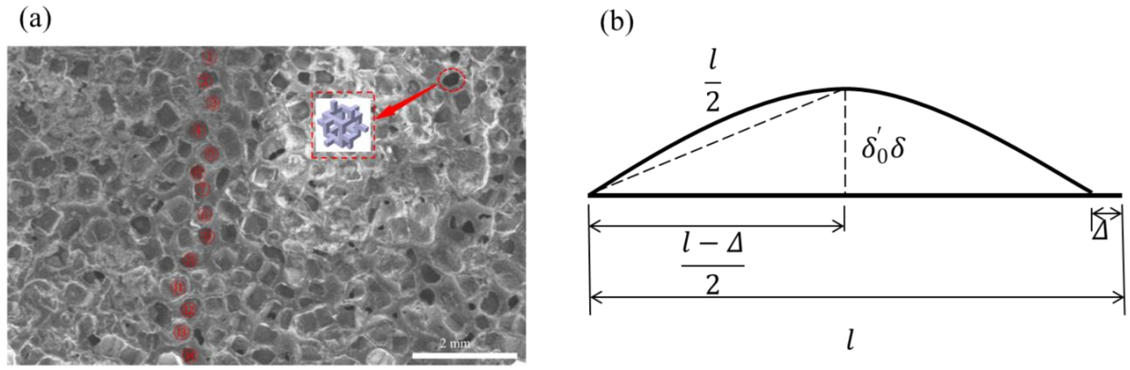

Supplementary Fig. 4. (a) SEM image of porous PDMS, (b) The schematic calculation model of the ligament.

## Supplementary References

[1] J. Si *et al.*, “Characterization of 3D elastic porous polydimethylsiloxane (PDMS) cell scaffolds fabricated by VARTM and particle leaching,” *J. Appl. Polym. Sci.*, 2016, doi: 10.1002/app.42909.

[2] A. Rinaldi, et al., “A flexible and highly sensitive pressure sensor based on a PDMS foam coated with graphene nanoplatelets,” *Sensors (Switzerland)*, 2016, doi: 10.3390/s16122148.

[3] F. Chen *et al.*, “Table Salt as a Template to Prepare Reusable Porous PVDF–MWCNT Foam for Separation of Immiscible Oils/Organic Solvents and Corrosive Aqueous Solutions,” *Adv. Funct. Mater.*, 2017, doi: 10.1002/adfm.201702926.

[4] P. Martins, et al., “Electroactive phases of poly(vinylidene fluoride): Determination, processing and applications,” *Prog. Polym. Sci.*, 2014, doi: 10.1016/j.progpolymsci.2013.07.006.
